# Supplementary material for: Analyzing and Mitigating Inconsistency in Discrete Audio Tokens for Neural Codec Language Models
Source: arXiv:2409.19283 source file (2024-10-04)
Supplement: Supplementary file 1 [file 7_appendix.tex]

% You may include other additional sections here.

\subsection{Analysis of Inconsistencies Caused by Receptive Field Size}
\label{analysis_inconsistencies}

\begin{table}[!ht]
    \centering
    \caption{The parameters of the convolutional layers and the receptive field size in codec's encoder.}
    \scalebox{1.0}{
    \begin{tabular}{c|c|c|c|c|c}
    \hline
        \multirow{2}{*}{layer id} & \multirow{2}{*}{kernel size} & \multirow{2}{*}{stride} & \multirow{2}{*}{dilation} & \multirow{2}{*}{\makecell[c]{strides of \\ previous layers}} & \multirow{2}{*}{receptive field size} \\ 
        & & & & & \\ \toprule
        1 & 7 & 1 & 1 & 0 & $7$ \\ \midrule
        2 & 3 & 1 & 1 & 1 & $7+(3-1)\times1=9$ \\ \midrule
        3 & 1 & 1 & 1 & 1 & $9+(1-1)\times1=9$ \\ \midrule
        4 & 1 & 1 & 1 & 1 & $9+(1-1)\times1=9$ \\ \midrule
        5 & 4 & 2 & 1 & 1 & $9+(4-1)\times1=12$ \\ \midrule
        6 & 3 & 1 & 1 & 2 & $12+(3-1)\times2=16$ \\ \midrule
        7 & 1 & 1 & 1 & 2 & $16+(1-1)\times2=16$ \\ \midrule
        8 & 1 & 1 & 1 & 2 & $16+(1-1)\times2=16$ \\ \midrule
        9 & 8 & 4 & 1 & 2 & $16+(8-1)\times2=30$ \\ \midrule
        10 & 3 & 1 & 1 & 8 & $30+(3-1)\times8=46$ \\ \midrule
        11 & 1 & 1 & 1 & 8 & $46+(1-1)\times8=46$ \\ \midrule
        12 & 1 & 1 & 1 & 8 & $46+(1-1)\times8=46$ \\ \midrule
        13 & 10 & 5 & 1 & 8 & $46+(10-1)\times8=118$ \\ \midrule
        14 & 3 & 1 & 1 & 40 & $118+(3-1)\times40=198$ \\ \midrule
        15 & 1 & 1 & 1 & 40 & $198+(1-1)\times40=198$ \\ \midrule
        16 & 1 & 1 & 1 & 40 & $198+(1-1)\times40=198$ \\ \midrule
        17 & 16 & 8 & 1 & 40 & $198+(16-1)\times40=798$ \\ \midrule
        18 & 7 & 1 & 1 & 320 & $798+(7-1)\times320=2718$ \\ \hline
    \end{tabular}}
    \label{receptive_field}
\end{table}

The size of the receptive field is influenced by convolutional layers and pooling layers, whereas activation functions and batch normalization do not affect it. The stride of the current layer does not impact its receptive field. The method to calculate the receptive field of the current layer is
$$RF_i = RF_{i-1} + (k - 1) \times S_i$$
where \(RF_i\) represents the receptive field of the current layer, and \(RF_{i-1}\) denotes the receptive field size of the previous layer. \(S_i\) represents the product of the strides of all previous layers (excluding the current layer), and is given by:
$$S_i = \prod_{i=1}^{L_i} stride_i$$
Table \ref{receptive_field} presents the parameters of the convolutional layers in the encoders of codec and ConsistencyCodec. After calculations, the receptive field size of the final layer of the encoder is determined to be 2718. This indicates that when the audio is discretized into discrete units by the codec, each discrete unit's context includes 2718 audio samples.

% \textbf{Encoder and decoder architecture} 

\subsection{Training object}

The overall training objective consists of five components: reconstruction loss, adversarial loss, feature matching loss, RVQ commit loss, and the consistency loss.

\begin{center}
\begin{aligned}
\mathcal{L}_{f}(x, \hat{x}) & =\frac{1}{|\alpha|} \sum_{i \in \alpha}\left(\left\|\mathcal{S}_{i}(x)-\mathcal{S}_{i}(\hat{x})\right\|_{1}+\left\|\mathcal{S}_{i}(x)-\mathcal{S}_{i}(\hat{x})\right\|_{2}\right. \\
& \left.+\left\|\mathcal{M}_{i}(x)-\mathcal{M}_{i}(\hat{x})\right\|_{1}+\left\|\mathcal{M}_{i}(x)-\mathcal{M}_{i}(\hat{x})\right\|_{2}\right)
\end{aligned}
\end{center}

\begin{equation*}
\mathcal{L}_{\text{adv}} (\hat{x}) = \mathbb{E}_{\hat{x}} \left[ \frac{1}{K} \sum_{k,t} \frac{1}{T_k} \max(0, 1 - D_{k, t}(\hat{x})) \right]
\end{equation*}

\begin{equation*}
\mathcal{L}_{\text{feat}} (x, \hat{x}) = \mathbb{E}_{x, \hat{x}} \left[ \frac{1}{KL} \sum_{k,t,l} \frac{1}{T_k} \left\| D^{(l)}_{k, t} (x) - D^{(l)}_{k, t} (\hat{x}) \right\|_1 \right]
\end{equation*}

\begin{equation*}
\mathcal{L}_{\text{cm}} = \| V - \text{RVQ}(V) \|_2 + \frac{1}{N} \sum_{i} \| Q_{i-1} - \text{VQ}(Q_{i-1}) \|_2
\end{equation*}

% \mathcal{L} = \lambda_{t} \mathcal{L}_{t} + \lambda_{f} \mathcal{L}_{f} + \lambda_{\text{adv}} \mathcal{L}_{\text{adv}} + \lambda_{\text{feat}} \mathcal{L}_{\text{feat}} + \lambda_{\text{cm}} \mathcal{L}_{\text{cm}}

and the total loss

$$
\mathcal{L} = \mathcal{L}_{\mathrm{rec}} + \lambda_{\mathrm{adv}} \mathcal{L}_{\mathrm{adv}} + \lambda_{\mathrm{fm}} \mathcal{L}_{\mathrm{fm}} + \lambda_{\mathrm{rvq}} \mathcal{L}_{\mathrm{rvq}} + 
\lambda_{\mathrm{con}} \mathcal{L}_{\mathrm{consistency}}
$$

\subsection{Consistency accuracy of each layer}
% \cline{2-9}\rule{0pt}{16pt}
% \cmidrule(l){2-9}
\begin{table}[!ht]
    \centering
    \caption{Consistency accuracy of each of the first 8 layers within the neural audio codec.}
    \scalebox{0.9}{
    \begin{tabular}{c|ccc|cccccccc}
        \toprule
        \multirow{3}{*}{codec} & \multicolumn{8}{c}{every layer's consistency} \\ \cline{2-9}\rule{0pt}{16pt} 
        & 1 & 2 & 3 & 4 & 5 & 6 & 7 & 8 \\
        \midrule
        EnCodec & 90.57\% & 83.43\% & 77.15\% & 71.20\% & 65.68\% & 60.45\% & 54.08\% & 49.41\% \\
        FunCodec & 38.73\% & 17.68\% & 10.66\% & 7.73\% & 5.46\% & 5.25\% & 3.34\% & 1.85\% \\
        HiFiCodec & 77.71\% & 76.09\% & 41.61\% & 41.72\% & / & / & / & / \\
        SpeechTokenizer & 69.42\% & 47.55\% & 36.72\% & 27.71\% & 21.13\% & 16.39\% & 13.67\% & 11.38\% \\
        ConsistencyCodec & 97.87\% & 94.88\% & 91.36\% & 87.02\% & 82.70\% & 77.83\% & 71.92\% & 67.25\% \\
        \bottomrule
    \end{tabular}
    }
    \label{every_layer_consistency}
\end{table}

\subsection{Evaluation baselines}
\label{appendix_baseline}
1. \textbf{SpeechGPT}\citep{zhang2023speechgpt} is a large language model with conversational abilities, capable of perceiving and generating text and speech content. It uses HuBERT to encodec speech into semantic tokens, which are then deduplicated and used as input and output for the speech modality.

2. \textbf{USLM}\citep{zhang2023speechtokenizer} is built upon SpeechTokenizer and consists of both autoregressive and non-autoregressive models to hierarchically model information in speech. The autoregressive model captures the content information, while the non-autoregressive model complements it by adding paralinguistic information.

3. \textbf{AnyGPT}\citep{zhan2024anygpt} is an any-to-any multimodal language model that utilizes discrete representations for the unified processing of various modalities, including speech, text, images, and music. It also uses SpeechTokenizer to quantize speech.

4. \textbf{VoiceCraft}\citep{peng2024voicecraft} is a token-infilling neural codec language model. It introduces a token rearrangement procedure that combines causal masking and delayed stacking to enable generation within an existing sequence.

5. \textbf{XTTS v2}\citep{casanova2024xtts} is a massively multilingual text-to-speech (TTS) model and takes a mel-spectrogram as input. During training, it uses VQ-VAE to discretize the mel-spectrogram with a codebook consisting of 8192 codes. After training, it filters and retains the most common 1024 codewords.

6. \textbf{VALL-E} reproduced by Amphion\citep{zhang2023amphion} also adopts SpeechTokenizer as the neural audio codec.

\subsection{Explore different configurations of consistency constraint strategy}
\begin{table}[!ht]
    \centering
    \caption{The zero-shot TTS evaluation results for VALL-E, with 44K hours training data. \textbf{Bold} for the best result, and \underline{underline} for the second-best result.}
    \scalebox{0.9}{
    \begin{tabular}{ccc|ccc|cc}
        \toprule
        \multicolumn{3}{c|}{\multirow{2}{*}{codec config}} & \multicolumn{3}{c|}{\multirow{2}{*}{Objective}} & \multicolumn{2}{c}{\multirow{2}{*}{Subjective}}\\
        & & & & & & &\\
        \cline{1-8}\rule{0pt}{16pt}
        bandwidth & \makecell[c]{slice\\percentage} & perturb method & WER↓ & SIM↑ & UTMOS↑ & SMOS↑ & MOS↑ \\
        \midrule
        \multirow{4}{*}{2.0 kbps} & / & / & 8.67 & 72.34\% & 4.07 & 4.24 & 4.04\\ \cmidrule(lr){2-8}
        & {20\%} & phase perturb & 5.98 & 74.66\% & 4.10 & 4.31 & 4.12\\ \cmidrule(lr){2-8}
        & {40\%} & phase perturb & 6.57 & 74.84\% & 4.07 & 4.28 & 4.01\\
        \midrule
        \multirow{4}{*}{4.0 kbps} & / & / & 5.51 & 83.58\% & 4.13 & 4.40 & 3.99\\ \cmidrule(lr){2-8}
        & {20\%} & phase perturb & \textbf{3.85} & \textbf{87.24\%} & \textbf{4.32} & \textbf{4.46} & \textbf{4.16}\\ \cmidrule(lr){2-8}
        & {40\%} & phase perturb & \underline{4.71} & \underline{85.48\%} & \underline{4.28} & \underline{4.42} & \underline{4.11}\\
        \bottomrule
    \end{tabular}
    }
    \label{tab:valle_44kh}
\end{table}
